# Supplementary material for: Analyzing Emissions and Energy Efficiency at Unsignalized Real-world Intersections Under Mixed Traffic Control
Source: arXiv:2311.11866 source file (2024-01-17)
Supplement: Supplementary file 1 [file appendix.tex]

\section*{APPENDIX}
